# Supplementary material for: Field theory for amorphous solids
Source: arXiv:1808.01811 source file (2018-08-06)
Supplement: Supplementary file 1 [file FieldTheory_SI.pdf]

# Field theory for amorphous solids – Supplementary Information

E. DeGiuli
*Institut de Physique Théorique Philippe Meyer, École Normale Supérieure, PSL University, Sorbonne Universités, CNRS, 75005 Paris, France*

Here we give a schematic derivation of the sampling probability for stress in fluctuations about a metastable state, for a material which can be treated as elastic. We will see through this construction the effect of finite temperature.

Consider an elastic material fluctuating about a metastable state. Its Piola-Kirchoff stress tensor is [1]

$$\hat{\sigma} = \hat{\bar{\sigma}} + \mu \nabla \vec{u} + \mu (\nabla \vec{u})^t + \lambda \hat{\delta} \nabla \cdot \vec{u}, \tag{1}$$

where $\hat{\bar{\sigma}}(\vec{r})$ is the mechanically-equilibrated pre-stress, thus satisfying $\nabla \cdot \hat{\bar{\sigma}} = 0$. The elastic energy is

$$H = \int dV \; \tfrac{1}{2} \hat{\sigma}[u] : \big( \nabla \vec{u} + (\nabla \vec{u})^t + \nabla \vec{u} \cdot (\nabla \vec{u})^t \big), \tag{2}$$

including the nonlinear displacement term, which couples to the pre-stress [1]. A simple model for the sampling probability of $\hat{\bar{\sigma}}$ is obtained by integrating the Boltzmann measure over the elastic fluctuations:

$$\omega[\hat{\bar{\sigma}}] = \int Du \; e^{-\beta H}, \tag{3}$$

Keeping terms quadratic in displacement, this can be written in Fourier space as

$$H = \int d^d q \int d^d q' \; \vec{u}(\vec{q}) \cdot \hat{K}(\vec{q}, \vec{q}\,') \cdot \vec{u}(\vec{q}\,') \tag{4}$$

where the kernel is

$$\hat{K}(\vec{q}, \vec{q}\,') = \hat{A} \delta(\vec{q} - \vec{q}\,') - \hat{\delta} \, \hat{\bar{\sigma}}(\vec{q} + \vec{q}\,')^{\dagger} : \vec{q} \vec{q}\,' \tag{5}$$

with $\hat{A} = (\lambda + \mu) \vec{q} \vec{q}\,' + \mu q^2 \hat{\delta}$. The terms linear in $\vec{u}$ have vanished from mechanical equilibrium, up to boundary terms that we neglect here. In this harmonic approximation, we have

$$\omega[\hat{\bar{\sigma}}] \propto |K|^{-1/2} = e^{-\frac{1}{2} Tr \log K}, \tag{6}$$

which is independent of temperature. Assuming that the elastic moduli are much larger than the applied stress, the functional determinant can be expanded as

$$Tr \log K = Tr \log \hat{A} \delta(\vec{q} - \vec{q}\,') - Tr(\hat{A}^{-1} \hat{\bar{\sigma}}(\vec{q} + \vec{q}\,')^{\dagger} : \vec{q} \vec{q}\,') + \tfrac{1}{2} Tr(\hat{A}^{-1} \hat{\bar{\sigma}}(\vec{q} + \vec{q}\,')^{\dagger} : \vec{q} \vec{q}\,' \hat{A}^{-1} \hat{\bar{\sigma}}(\vec{q}\,' + \vec{q})^{\dagger} : \vec{q}\,' \vec{q}) + \ldots \tag{7}$$

The Fourier integrals needed to evaluate the trace can be done, in principle. We see that a Landau-Wilson expansion of the measure on $\hat{\bar{\sigma}}$ is generated. At order $\hat{\bar{\sigma}}^n$, all terms will have a coefficient that scales as the elastic moduli to the $-n^{th}$ power.

What is the effect of temperature? Suppose that, in experiment, we measure the correlations of the total stress $\hat{\sigma}$. These will have a component from the displacement fluctuations. Consider for example $\langle \nabla \vec{u}(\vec{r}) (\nabla \vec{u}(\vec{r}\,'))^t \rangle_c$, which in Fourier space is given by

$$-\langle \vec{q} \, \vec{u}(\vec{q}) \vec{u}(\vec{q}\,')^{\dagger} \vec{q}\,' \rangle_c = -\frac{1}{\beta} \vec{q} \, \hat{K}(\vec{q}, \vec{q}\,')^{-1} \vec{q}\,' \tag{8}$$

in the harmonic approximation. We notice that these correlations are longitudinal, and proportional to $T$, as claimed in the main text. Expanding $\hat{K}^{-1}$ in $\hat{\bar{\sigma}}$, the leading term gives

$$-\langle \vec{q} \, \vec{u}(\vec{q}) \vec{u}(\vec{q}\,')^{\dagger} \vec{q}\,' \rangle_c = -\frac{1}{\beta} \delta(\vec{q} - \vec{q}\,') \vec{q} \left[ \frac{1}{\mu q^2} \big( \hat{\delta} - \frac{\vec{q}\vec{q}}{q^2} \big) + \frac{1}{\lambda + 2\mu} \frac{\vec{q}\vec{q}}{q^4} \right] \vec{q}\,' + \ldots \tag{9}$$

This has nonanalytic dependence on $\vec{q}/q$, giving some angular dependence in real-space, but is short-range. Higher-order terms in $\hat{\bar{\sigma}}$ will however have longitudinal, long-range dependence. Other contributions to the correlator will behave similarly, and mixed transverse-longitudinal correlators will vanish up to total derivatives.

This construction is schematic for several reasons: first, we assume that the material is fluctuating elastically about its metastable state, which may not be a good model for granular matter, for example; second, to obtain

tractable results, we need to assume that the pre-stress is small compared to the elastic moduli; and finally, the Fourier integrals may need regularization, especially in $d = 2$.

[1] B. DiDonna and T. Lubensky, Physical Review E **72**, 066619 (2005).
